# Supplementary material for: A Stochastic Derivative-Free Optimization Method with Importance Sampling: Theory and Learning to Control
Source: arXiv:1902.01272 source file (2020-04-02)
Supplement: Supplementary file 2 [file nonconvex.tex]

\section{Non convex case}

\begin{thm} Let Assumption~\ref{ass:M-smooth} hold. Choose $\alpha_{i_k}=\tfrac{\alpha_0}{v_{i_k} \sqrt{k+1}}$, where $\alpha_0>0$. If
\begin{equation}\label{eq:isjss8sus-} 
K\geq \frac{2 \left( \frac{\sqrt{2}(f(x_0)-f_*)}{\alpha_0} + \frac{\alpha_0 \sum_{i=1}^n  \frac{p_i {L_i}}{{v_{i}^2}}}{2} \right)^2}{\left(\min_i \frac{p_i}{v_i}\right)^2 \epsilon^2},
\end{equation}
then $\displaystyle \min_{k=0,1,\dots,K} \mathbb{E} \left[ \|\nabla f(x_k)\|_{1} \right] \leq \epsilon.$
\end{thm}
\begin{proof}
We have from Lemma~\ref{lemma:key_lem} 
\begin{equation} \label{eq:condexp}
\mathbb{E} \left[ f(x_{k+1}) \;|\; x_k \right] \leq f(x_k)-  \underbrace{\mathbb{E} \left[ \alpha_{i_k} |\ve{ \nabla f(x_k)}{e_{i_k}}| \;|\; x_k \right]}_{\circledOne} + \underbrace{\frac{1}{2} \mathbb{E} \left[\alpha_{i_k}^2 L_{i_k} \;|\; x_k\right]}_{\circledTwo},
\end{equation}

From \circledOne we have 
\begin{eqnarray*}
\mathbb{E} \left[ \alpha_{i_k} |\ve{\nabla f(x_k)}{e_{i_k}}| \;|\; x_k \right] &= \frac{\alpha_0}{\sqrt{k+1}} \sum_{i=1}^n \frac{p_i}{{v_{i}}} |\ve{\nabla f(x_k)}{e_{i_k}}| \ge \frac{\alpha_0}{\sqrt{k+1}} \min_i\frac{p_i}{v_i} \|\nabla f(x_k)\|_1.
\end{eqnarray*}

From \circledTwo we have
\begin{eqnarray*}
\frac{1}{2} \mathbb{E} \left[ \alpha_{i_k}^2 L_{i_k} | x_k \right] &= &\frac{1}{2} \frac{\alpha_0^2}{{k+1}} \sum_{i=1}^n \frac{p_i {L_i}}{{v_{i}^2}}
\end{eqnarray*}

By injecting \circledOne and \circledTwo in (\ref{eq:condexp}) and taking the expectation we get 
\begin{equation} 
\theta_{k+1}  \leq \theta_{k} - \frac{\alpha_0 \min_i\frac{p_i}{v_i}}{ \sqrt{k+1}} g_k  + \frac{\alpha_0^2 \sum_{i=1}^n \frac{p_i L_i}{v_i^2}}{2({k+1})},
\end{equation}
where $\theta_{k} = \mathbb{E} \left[ f(x_k) \right]$  and $g_k = \mathbb{E} \left[ \|\nabla f(x_k)\|_1 \right]$. By re-arranging the terms we get:

\begin{equation}
\label{eq:s9jd7d76d-} 
g_k \leq   \frac{1}{\min_i \frac{p_i}{v_i}} \left( \frac{(\theta_k-\theta_{k+1})\sqrt{k+1}}{\alpha_0} + \frac{\alpha_0 \sum_{i=1}^n \frac{p_i L_i}{v_i^2}}{2 \sqrt{k+1}}\right).
\end{equation}

We have that the sequence $\left\{f(x_k)\right\}_{k\ge 0}$ is monotonically decreasing and  $f$ is bounded from below by $f(x_*)$, hence $f(x_*) \leq \theta_{k+1}\leq \theta_k\leq f(x_0)$ for all $k$. Letting $l=\lfloor K/2 \rfloor$, this implies that \[\sum_{j=l}^{2l} \theta_{j}-\theta_{j+1}  = \theta_l - \theta_{2l+1} \leq  f(x_0)-f(x_*)\eqdef C,\]
from which we conclude that there must exist $j\in \{l,\dots,2l\}$ such that $\theta_j-\theta_{j+1}\leq C/(l+1)$. This implies that
\begin{eqnarray*}
g_j &\overset{\eqref{eq:s9jd7d76d-}}{\leq} & \frac{1}{\min_i \frac{p_v}{v_i}} \left( \frac{(\theta_j-\theta_{j+1})\sqrt{j+1}}{\alpha_0} + \frac{\alpha_0 \sum_{i=1}^n \frac{p_i L_i}{v_i^2}}{2 \sqrt{j+1}}\right)\\
&\leq &  \frac{1}{\min_i \frac{p_v}{v_i}} \left( \frac{C\sqrt{j+1}}{\alpha_0 (l+1)} + \frac{\alpha_0 \sum_{i=1}^n \frac{p_i L_i}{v_i^2}}{2 \sqrt{j+1}}\right)\\
&\leq &  \frac{1}{\min_i \frac{p_v}{v_i}} \left( \frac{C\sqrt{2l+1}}{\alpha_0 (l+1)} + \frac{\alpha_0 \sum_{i=1}^n \frac{p_i L_i}{v_i^2}}{2 \sqrt{l+1}}\right)\\
&\leq & \frac{1}{\min_i \frac{p_v}{v_i} \sqrt{l+1}} \left( \frac{\sqrt{2}C}{\alpha_0 } + \frac{\alpha_0 \sum_{i=1}^n \frac{p_i L_i}{v_i^2}}{2}\right)\\
&\leq & \frac{1}{\min_i \frac{p_v}{v_i} \sqrt{K/2}} \left( \frac{\sqrt{2}C}{\alpha_0 } + \frac{\alpha_0 \sum_{i=1}^n \frac{p_i L_i}{v_i^2}}{2}\right)\\
&\overset{\eqref{eq:isjss8sus-}}{\leq} & \epsilon.
\end{eqnarray*}
\end{proof}

\begin{thm} Let Assumption \ref{ass:M-smooth} be satisfied. Choose $\alpha_{i_k}= \frac{\epsilon}{n v_{{i_k}}}$ where $\sum_{i=1}^n \frac{p_i L_i}{v_i^2} < 2n \left(\min_i \frac{p_i}{v_i}\right)$. If
\begin{equation} \label{eq:isjss8sus-2}
   K \ge    \frac{2 n \left(f(x_0)-f(x_*)\right)}{\min_i \frac{p_i}{v_i} \left(1 -\frac{\sum_{i=1}^n  \frac{p_i {L_i}}{{v_{i}^2}}}{2n \min_i \frac{p_i}{v_i}} \right)  \epsilon^2},
\end{equation}
then  $\displaystyle \min_{k=0,1,\dots,K} \mathbb{E} \left[ \|\nabla f(x_k)\|_{1} \right] \leq \epsilon$.
\end{thm}
\begin{proof}  
From equation (\ref{eq:condexp}) we have 
\begin{eqnarray}\label{eq:condexp-}
\mathbb{E} \left[ f(x_{k+1}) \;|\; x_k \right] &\leq& f(x_k)-  \underbrace{\mathbb{E} \left[ \alpha_{i_k} |\ve{\nabla f(x_k)}{e_{i_k}}| \;|\; x_k  \right]}_{\circledOne} + \underbrace{\frac{1}{2} \mathbb{E} \left[ \alpha_{i_k}^2 L_{i_k} \right]}_{\circledTwo}.
\end{eqnarray}

From \circledOne we have 
\begin{eqnarray*}
\mathbb{E} \left[ \alpha_{i_k} |\ve{\nabla f(x_k)}{e_{i_k}}| \;|\; x_k \right] &=& \frac{\epsilon}{n} \sum_{i=1}^n \frac{p_i}{{v_{i}}} |\ve{\nabla f(x_k)}{e_{i_k}}| \\
&\ge& \frac{\epsilon \min_i \frac{p_i}{v_i}}{ n} \|\nabla f(x_k)\|_1.
\end{eqnarray*}

From \circledTwo we have
\begin{eqnarray*}
\frac{1}{2} \mathbb{E} \left[ \alpha_{i_k}^2 L_{i_k} \right] &= &\frac{1}{2} \frac{\epsilon^2}{n^2} \sum_{i=1}^n \frac{p_i {L_i}}{{v_{i}^2}} 
\end{eqnarray*}
By injecting \circledOne and \circledTwo in (\ref{eq:condexp-}) and taking the expectation we get 
\begin{equation} 
\theta_{k+1}  \leq \theta_{k} - \frac{\epsilon}{n} \min_i \frac{p_i}{v_i} g_k  + \frac{\epsilon^2}{2 n^2}\sum_{i=1}^n \frac{p_i {L_i}}{{v_{i}^2}},
\end{equation}
where $\theta_{k} = \mathbb{E} \left[ f(x_k) \right]$  and $g_k = \mathbb{E} \left[ \|\nabla f(x_k)\|_1 \right]$. By re-arranging the terms we get:

\begin{equation}
\label{eq:s9jd7d76d} 
g_k \leq    \left( \frac{(\theta_k-\theta_{k+1})n }{\epsilon \min_i \frac{p_i}{v_i}} + \frac{\epsilon \sum_{i=1}^n \frac{p_i {L_i}}{{v_{i}^2}}}{2 n \min_i \frac{p_i}{v_i}}\right).
\end{equation}
We have that the sequence $\left\{f(x_k)\right\}_{k\ge 0}$ is monotonically decreasing and  $f(x)$ is bounded from below by $f(x_*)$, hence $f(x_*)\leq \theta_{k+1}\leq \theta_k\leq f(x_0)$ for all $k$. Letting $l=\lfloor K/2 \rfloor$, this implies that \[\sum_{j=l}^{2l} \theta_{j}-\theta_{j+1}  = \theta_l - \theta_{2l+1} \leq  f(x_0)-f(x_*) = C,\]
from which we conclude that there must exist $j\in \{l,\dots,2l\}$ such that $\theta_j-\theta_{j+1}\leq C/(l+1)$.
This implies that
\begin{eqnarray*}
g_k &\leq&    \left( \frac{C n }{\epsilon \min_i \frac{p_i}{v_i} (l+1)} + \frac{\epsilon \sum_{i=1}^n \frac{p_i {L_i}}{{v_{i}^2}}}{2 n \min_i \frac{p_i}{v_i}}\right)\\
&\leq& \left( \frac{C n }{\epsilon \min_i \frac{p_i}{v_i} K/2} + \frac{\epsilon \sum_{i=1}^n \frac{p_i {L_i}}{{v_{i}^2}}}{2 n \min_i \frac{p_i}{v_i}}\right)\\
&\overset{\eqref{eq:isjss8sus-2}}{\leq}&  \epsilon.
\end{eqnarray*}
\end{proof}
